# Supplementary material for: The critical Karp--Sipser core of Erd\H{o}s--R\'enyi random graphs
Source: arXiv:2412.04328 ancillary file (2024-12-05)
Supplement: Supplementary file 1 [file computations.pdf]

## Definition of the functions

```
In[1]:= f[z_] := E^z - 1 - z
In[2]:= PhiA[x_, v_, s_, z_] := -1 - x / (x + 2 v + s) + v^2 z^4 E^z / ((x + 2 v + s)^2 f[z]^2) -
      x v z^2 E^z / ((x + 2 v + s)^2 f[z]); PhiB[x_, v_, s_, z_] :=
      -1 + x / (x + 2 v + s) - v^2 z^4 E^z / ((x + 2 v + s)^2 f[z]^2);
PhiC[x_, v_, s_, z_] := 1 - x / (x + 2 v + s) - 2 v z^2 E^z / ((x + 2 v + s) f[z]) +
      v^2 z^4 E^z / ((x + 2 v + s)^2 f[z]^2) + x v z^2 E^z / ((x + 2 v + s)^2 f[z]);
```

## Lemma 7: Asymptotics of the derivatives near the end

We compute the derivative of PhiA with respect to x, where z is an implicit parameter characterized by  $z(E^z - 1)/f[z] = 2 + s/v$

```
In[4]:= ImplicitD[PhiA[x, v, s, z], z (E^z - 1) / f[z] == 2 + s / v, z, x] // FullSimplify
```

```
Out[4]= - 
$$\frac{1}{(s + 2v + x)^3 (1 - e^z + z)^2} \left( s^2 (1 - e^z + z)^2 + s (-1 + e^z - z) \left( -((4v + x)(1 + z)) + e^z (x + v(4 + z^2)) \right) + \right. \\ \left. v (x(1 - e^z + z)(2(1 + z) + e^z(-2 + z^2)) + 2v(2(1 + z)^2 + e^{2z}(2 + z^2) + e^z(-4 + z(-4 + z(-1 + (-1 + z)z)))) \right)$$

```

We compute the three derivatives of PhiA with respect to x, v and s respectively, parametrize them using  $\beta$  and then compute their series expansion at  $\beta = \left(\frac{1}{e}\right)^-$

```
In[5]:= Series[{ImplicitD[PhiA[x, v, s, z], z (E^z - 1) / f[z] == 2 + s / v, z, x],
      ImplicitD[PhiA[x, v, s, z], z (E^z - 1) / f[z] == 2 + s / v, z, v],
      ImplicitD[PhiA[x, v, s, z], z (E^z - 1) / f[z] == 2 + s / v, z, s]} /.
      v -> beta E^(-z) f[z] /. x -> z^2 / E - z beta (1 - E^(-z)) /.
      s -> beta (z + z E^(-z) + 2 E^(-z) - 2) /. z -> E beta + Log[beta],
      {beta, 1 / E, -1}, Direction -> "FromBelow"] // FullSimplify
```

```
Out[5]= 
$$\left\{ -\frac{1}{e \left(\beta - \frac{1}{e}\right)^2} - \frac{3}{4 \left(\beta - \frac{1}{e}\right)} + 0 \left[\beta - \frac{1}{e}\right]^0, \right. \\ \left. 0 \left[\beta - \frac{1}{e}\right]^0, -\frac{1}{2 \left(\beta - \frac{1}{e}\right)} + 0 \left[\beta - \frac{1}{e}\right]^0 \right\}$$

```

Recall that  $\beta - e^{-1} = e^{-1/2} \epsilon^{1/2} + \frac{5}{12} \epsilon + O(\epsilon^{3/2})$ . The second derivative (the one with respect to v) is  $O(1)$ . We replace beta as a function of epsilon in the first and third term.

```
In[6]:= Series[{- $\frac{1}{e \left(\beta - \frac{1}{e}\right)^2} - \frac{3}{4 \left(\beta - \frac{1}{e}\right)} + O[\text{eps}]^0$ ,  $-\frac{1}{2 \left(\beta - \frac{1}{e}\right)} + O[\text{eps}]^0$ } /.
  beta  $\rightarrow 1/E + E^{(-1/2)} \text{eps}^{(1/2)} + 5/12 \text{eps} + C \text{eps}^{(3/2)}$ ,
  {eps, 0, -1}, Direction  $\rightarrow$  "FromBelow"] // FullSimplify

Out[6]=  $\left\{-\frac{1}{\text{eps}} + \frac{1}{\sqrt{O[\text{eps}]}} , \frac{1}{\sqrt{O[\text{eps}]}}\right\}$ 
```

This gives the first three derivatives of Lemma 7. Let us move on to PhiB

```
In[7]:= Series[{ImplicitD[PhiB[x, v, s, z], z (E^z - 1) / f[z] == 2 + s / v, z, x],
  ImplicitD[PhiB[x, v, s, z], z (E^z - 1) / f[z] == 2 + s / v, z, v],
  ImplicitD[PhiB[x, v, s, z], z (E^z - 1) / f[z] == 2 + s / v, z, s]} /.
  v  $\rightarrow \beta E^{(-z)} f[z] /. x \rightarrow z^2/E - z \beta (1 - E^{(-z)}) /.
  s \rightarrow \beta (z + z E^{(-z)} + 2 E^{(-z)} - 2) /. z \rightarrow E \beta + \text{Log}[\beta]$ ,
  {beta, 1/E, -2}, Direction  $\rightarrow$  "FromBelow"] // FullSimplify

Out[7]=  $\left\{\frac{3}{4 e \left(\beta - \frac{1}{e}\right)^2} + \frac{1}{O\left[\beta - \frac{1}{e}\right]}, \frac{1}{O\left[\beta - \frac{1}{e}\right]}, \frac{1}{O\left[\beta - \frac{1}{e}\right]}\right\}$ 
```

The second and third terms are  $O(1/(\beta - 1/e)) = O(\epsilon^{-1/2})$ . For the first term, replacing  $\beta$  as a function of  $\epsilon$ , we obtain

```
In[8]:= Series[ $\frac{3}{4 e \left(\beta - \frac{1}{e}\right)^2} /.
  beta \rightarrow 1/E + E^{(-1/2)} \text{eps}^{(1/2)} + 5/12 \text{eps} + C \text{eps}^{(3/2)}$ ,
  {eps, 0, -1}, Direction  $\rightarrow$  "FromBelow"] // FullSimplify

Out[8]=  $\frac{3}{4 \text{eps}} + \frac{1}{\sqrt{O[\text{eps}]}}$ 
```

We finally move to the derivation of PhiC.

```
In[9]:= Series[{ImplicitD[PhiC[x, v, s, z], z (E^z - 1) / f[z] == 2 + s / v, z, x],
  ImplicitD[PhiC[x, v, s, z], z (E^z - 1) / f[z] == 2 + s / v, z, v],
  ImplicitD[PhiC[x, v, s, z], z (E^z - 1) / f[z] == 2 + s / v, z, s]} /.
  v  $\rightarrow \beta E^{(-z)} f[z] /. x \rightarrow z^2/E - z \beta (1 - E^{(-z)}) /.
  s \rightarrow \beta (z + z E^{(-z)} + 2 E^{(-z)} - 2) /. z \rightarrow E \beta + \text{Log}[\beta]$ ,
  {beta, 1/E, 0}, Direction  $\rightarrow$  "FromBelow"] // FullSimplify

Out[9]=  $\left\{\frac{3}{4 \left(\beta - \frac{1}{e}\right)} + \frac{29 e}{48} + O\left[\beta - \frac{1}{e}\right]^1, \frac{1}{\beta - \frac{1}{e}} + \frac{5 e}{4} + O\left[\beta - \frac{1}{e}\right]^1,
  -\frac{3}{2 e \left(\beta - \frac{1}{e}\right)^2} - \frac{7}{4 \left(\beta - \frac{1}{e}\right)} + \frac{37 e}{160} + O\left[\beta - \frac{1}{e}\right]^1\right\}$ 
```

The first term is  $O(\epsilon^{-1/2})$ . For the last two terms, replacing  $\beta$  as a function of  $\epsilon$ , we obtain

```
In[10]:= {Series[ $\frac{1}{\text{beta} - \frac{1}{e}} + \frac{5e}{4}$  /.
    beta  $\rightarrow 1/E + E^{(-1/2)} \text{eps}^{(1/2)} + 5/12 \text{eps} + C \text{eps}^{(3/2)}$ , {eps, 0, 0},
    Direction  $\rightarrow$  "FromBelow"], Series[- $\frac{3}{2e(\text{beta} - \frac{1}{e})^2} - \frac{7}{4(\text{beta} - \frac{1}{e})}$  /.
    beta  $\rightarrow 1/E + E^{(-1/2)} \text{eps}^{(1/2)} + 5/12 \text{eps} + C \text{eps}^{(3/2)}$ ,
    {eps, 0, -1}, Direction  $\rightarrow$  "FromBelow"]} // FullSimplify
```

```
Out[10]=  $\left\{ \frac{\sqrt{e}}{\sqrt{\text{eps}}} + \frac{5e}{6} + \sqrt{0[\text{eps}]}, -\frac{3}{2 \text{eps}} + \frac{1}{\sqrt{0[\text{eps}]}} \right\}$ 
```

Note that we do not need the term of constant order in the derivative with respect to  $v$

## Lemma 8: Last estimate

We write  $bx = x/v$  and  $bs = s/v$

```
In[11]:= PhiA[bx v, v, bs v, z] // FullSimplify
```

```
Out[11]=  $-1 + \frac{-bx(2 + bs + bx) + \frac{e^z z^4}{(1 - e^z + z)^2} + \frac{bx e^z z^2}{1 - e^z + z}}{(2 + bs + bx)^2}$ 
```

The expression does not depend on  $v$  and we thus define PsiA as follows

```
In[12]:= PsiA[bx_, bs_, z_] := PhiA[bx v, v, bs v, z] // FullSimplify
```

We compute its derivative with respect to  $bs$ , where again  $z$  is an implicit parameter

```
In[13]:= ImplicitD[PsiA[bx, bs, z], z (E^z - 1) / f[z] == 2 + bs, z, bs] // FullSimplify
```

```
Out[13]=  $\frac{1}{(2 + bs + bx)^3} \left( -\frac{2 z^4 (1 + z)}{(1 - e^z + z)^2} + \frac{2 z^2 (2 + bs + 2 bx + (2 + bs + 2 bx) z - z^2)}{-1 + e^z - z} + bx (2 + bs + bx - 2 (2 + bs + bx) z + 2 z^2) + \frac{(2 + bs + bx) e^{-z} z (bx + z) (-2 + e^z (2 + (-2 + z) z))}{2 + z^2 - 2 \text{Cosh}[z]} \right)$ 
```

Since  $z$  depends on  $bs$  and goes to 0 as  $bs$  goes to 0, we replace  $bs$  as function of  $z$  in the previous expression...

```
In[14]:= % /. bs -> z (E^z - 1) / f[z] - 2 // FullSimplify
```

```
Out[14]=
```

$$- \left( \left( e^{-z} (1 - e^z + z)^2 \right. \right. \\ \left. \left( e^z z^4 (2 + e^z (-2 + z) + z) + bx^2 (1 - e^z + z) (1 + e^z (-2 + e^z (1 - 2z) + z (2 + z + z^2))) \right) + \right. \\ \left. bx z (1 + e^z (-3 - e^{2z} + 5z^2 + z^3 (4 + z) + e^z (3 + z^2 (-5 + 2z)))) \right) \left. \right) / \\ \left( (bx + z + bx z - e^z (bx + z))^3 (2 + z^2 - 2 \operatorname{Cosh}[z]) \right)$$

*... and compute the limit when  $z \rightarrow 0$  and  $bx \rightarrow 0$*

```
In[15]:= Limit[%, {z -> 0, bx -> 0}]
```

```
Out[15]=
```

0
